# Supplementary material for: Adversarial Risk and Robustness: General Definitions and Implications for the Uniform Distribution
Source: arXiv:1810.12272 source file (2018-10-29)
Supplement: Supplementary file 1 [file Supplementary.tex]

\documentclass[10pt,letterpaper]{article}

\usepackage[margin=1.2in]{geometry}

\usepackage{amssymb,amsmath,amsthm}
\usepackage[makeroom]{cancel}

\input{macros}

\begin{document}
\title{Supplementary Material for Paper\\
Revisting Risk and Robustness under Adversarial Perturbations}
\author{}
\date{}
\maketitle

\appendix
\input{appendix}

\end{document}
